# Supplementary material for: Why This and Not That? A Collaborative Reflection Approach for Understanding Thought Coverage in Decision Making Support Dialog
Source: arXiv:2608.17054 source file (2026-10-04)
Supplement: Supplementary file 1 [file appendix_F_same_state.tex]

The five largest same-state groups: sets of pause moments sharing identical knowledge base state (dominant dimension, score gap, observation type) but exhibiting the most diverse taxonomy categories. Each group illustrates how participants in structurally similar situations interpret the same pattern in fundamentally different ways.

\vspace{6pt}
\noindent\textbf{Group 1:} Dominant dimension = \textit{internal}, score gap = 10, observation type = \textit{standard}. \textit{n} = 19 moments; 8 distinct taxonomy categories.

\begin{table}[!h]
\footnotesize
\centering
\begin{tabular*}{\columnwidth}{@{\extracolsep{\fill}}@{} p{0.10\columnwidth} p{0.36\columnwidth} p{0.46\columnwidth} @{}}
\toprule
\textbf{ID} & \textbf{Category} & \textbf{Interpretation (truncated)} \\
\midrule
56 & Emotional Driver & \textit{i do not share my feelings with many, so it's nice to talk about them now} \\
127 & Self-Diagnosed Focus & \textit{exploring why it's easiest to stay} \\
130 & No Accessible Reason & \textit{I really dont know} \\
190 & Emotional Driver & \textit{from growing up and wanting to make people happy} \\
213 & Decision Nature & \textit{I seem to focus less on lived and shared experiences and focus more on my emotio\textbackslash\ldots} \\
207 & Deliberate Prioritisation & \textit{I wanted to talk aobut my feelings} \\
248 & Emotional Driver & \textit{It's connected to the feeling of uncertainty and self worth.} \\
250 & Self-Diagnosed Focus & \textit{As Im trying to understand myself and feelings.} \\
253 & Self-Diagnosed Focus & \textit{Feel that I am being honest with my current feelings.} \\
263 & Emotional Driver & \textit{I just want to show someone the love I have to give} \\
269 & Self-Diagnosed Focus & \textit{Because my biggest concern is relating to how I feel about the situation} \\
275 & Deliberate Prioritisation & \textit{As I wouldn't really think about practicals restraints or real world world condi\textbackslash\ldots} \\
282 & Interaction Attribution & \textit{The bot encouraged me to open up and think about my feelings in a constructive w\textbackslash\ldots} \\
288 & Pattern Disputed & \textit{The first part is accurate the second half doesn't feel accurate} \\
289 & No Accessible Reason & \textit{No} \\
293 & Thinking Style & \textit{I suppose emotions are very powerful in my head} \\
295 & Thinking Style & \textit{just the way I am} \\
315 & Self-Diagnosed Focus & \textit{my feelings are perhaps shaped by experiences people have shared with me and als\textbackslash\ldots} \\
321 & Deliberate Prioritisation & \textit{External factors cannot be ignored, as they can play a role. but what's more imp\textbackslash\ldots} \\
\bottomrule
\end{tabular*}
\end{table}

\vspace{6pt}
\noindent\textbf{Group 2:} Dominant dimension = \textit{external}, score gap = 4, observation type = \textit{standard}. \textit{n} = 18 moments; 7 distinct taxonomy categories.

\begin{table}[!h]
\footnotesize
\centering
\begin{tabular*}{\columnwidth}{@{\extracolsep{\fill}}@{} p{0.10\columnwidth} p{0.36\columnwidth} p{0.46\columnwidth} @{}}
\toprule
\textbf{ID} & \textbf{Category} & \textbf{Interpretation (truncated)} \\
\midrule
66 & Deliberate Prioritisation & \textit{i like to talk through practical aspects because these are where most of the wei\textbackslash\ldots} \\
87 & Decision Nature & \textit{Because these are real-life situations that people experience in their day-to-da\textbackslash\ldots} \\
96 & Emotional Driver & \textit{guilt} \\
122 & Deliberate Prioritisation & \textit{i am not sure how past experiences are relevant in the case of owning a pet} \\
125 & Decision Nature & \textit{I was explaining the situation which is caused by outside constraints} \\
135 & Decision Nature & \textit{Again, out of necessity} \\
144 & Deliberate Prioritisation & \textit{Similar to before, I think your own personal experience is crucial when it comes\textbackslash\ldots} \\
185 & Deliberate Prioritisation & \textit{Because where you live is as important as what you do} \\
195 & Deliberate Prioritisation & \textit{other factors wouldn't contribute currently such as emotions, its a practical pr\textbackslash\ldots} \\
216 & Interaction Attribution & \textit{I dont feel the conversation has progressed to this stage yet} \\
239 & Deliberate Prioritisation & \textit{I feel I have already discussed this} \\
246 & Decision Nature & \textit{You have to be practical in being able to live on the money you earn} \\
272 & Deliberate Prioritisation & \textit{I think it's because I'm trying to understand the situation in a more practical \textbackslash\ldots} \\
274 & Deliberate Prioritisation & \textit{I focus on external factors because I want a practical understanding of the job.} \\
281 & Self-Diagnosed Focus & \textit{I think I hide my emotions as I feel like I have to be the one in my family that\textbackslash\ldots} \\
284 & Self-Diagnosed Focus & \textit{I think although I remain calm, internally I'm constantly thinking about what ev\textbackslash\ldots} \\
307 & Thinking Style & \textit{Live experience and my professional life that almost always looks at practical /\textbackslash\ldots} \\
306 & No Accessible Reason & \textit{No} \\
\bottomrule
\end{tabular*}
\end{table}

\pagebreak % Optional breaking control indicator for multi-column printing balance

\noindent\textbf{Group 3:} Dominant dimension = \textit{external}, score gap = 6, observation type = \textit{standard}. \textit{n} = 17 moments; 7 distinct taxonomy categories.

\begin{table}[!h]
\footnotesize
\centering
\begin{tabular*}{\columnwidth}{@{\extracolsep{\fill}}@{} p{0.10\columnwidth} p{0.36\columnwidth} p{0.46\columnwidth} @{}}
\toprule
\textbf{ID} & \textbf{Category} & \textbf{Interpretation (truncated)} \\
\midrule
60 & Deliberate Prioritisation & \textit{I don't know where you're getting other people's opinions from.} \\
106 & Deliberate Prioritisation & \textit{It's mostly the external factors like home life that are important here} \\
108 & Deliberate Prioritisation & \textit{It's definitely a mixed back of internal feelings and external factors!} \\
116 & Deliberate Prioritisation & \textit{My feelings about this topic are fairly simple, and there's a lot more interesti\textbackslash\ldots} \\
119 & Deliberate Prioritisation & \textit{It feels expected, since I deliberately focused on personal emotions in this pha\textbackslash\ldots} \\
155 & Self-Diagnosed Focus & \textit{I think I'm generally not unhappy so I'm much more focussed on external factors.\textbackslash\ldots} \\
165 & Decision Nature & \textit{I think we covered all the topics overall, but there are clearly some strong pra\textbackslash\ldots} \\
197 & Decision Nature & \textit{It is a practical problem} \\
258 & Deliberate Prioritisation & \textit{It's because it's only the practical constraints that I can't see a clear way th\textbackslash\ldots} \\
285 & Emotional Driver & \textit{I hate to dwell on my past.} \\
292 & Deliberate Prioritisation & \textit{This question was already asked. I don't need to be too emotional about starting\textbackslash\ldots} \\
294 & Deliberate Prioritisation & \textit{As explained, I don't need to be emotional about this. It's creating a business \textbackslash\ldots} \\
296 & Deliberate Prioritisation & \textit{The same reasons as before. In creating a business, you can't rely only on past \textbackslash\ldots} \\
301 & Thinking Style & \textit{I am fact / risk driven in decision making} \\
308 & Content-Level Response & \textit{I have started a business before} \\
309 & Thinking Style & \textit{Because thats the way my brain works} \\
311 & No Accessible Reason & \textit{Not at the minute} \\
\bottomrule
\end{tabular*}
\end{table}

\vspace{6pt}
\noindent\textbf{Group 4:} Dominant dimension = \textit{internal}, score gap = 6, observation type = \textit{standard}. \textit{n} = 20 moments; 6 distinct taxonomy categories.

\begin{table}[!h]
\footnotesize
\centering
\begin{tabular*}{\columnwidth}{@{\extracolsep{\fill}}@{} p{0.10\columnwidth} p{0.36\columnwidth} p{0.46\columnwidth} @{}}
\toprule
\textbf{ID} & \textbf{Category} & \textbf{Interpretation (truncated)} \\
\midrule
54 & Emotional Driver & \textit{it's something i remember and took courage and i feel pride in myself as i was p\textbackslash\ldots} \\
89 & Deliberate Prioritisation & \textit{i dont care about lessons from people that i know, they dont mean much to me} \\
90 & Deliberate Prioritisation & \textit{i opened up about my partner} \\
101 & Thinking Style & \textit{I can't change the past, I can only change what I do. I am mostly self-taught an\textbackslash\ldots} \\
107 & Deliberate Prioritisation & \textit{Well we decided to go down this route when we started the conversation, so I've \textbackslash\ldots} \\
112 & Deliberate Prioritisation & \textit{It is a decision about me and my life} \\
136 & Decision Nature & \textit{I think experiences from the past/from other stories were really instrumental to\textbackslash\ldots} \\
137 & Deliberate Prioritisation & \textit{Yes I agree- because this decision is mine and impacts me primarily, so I think \textbackslash\ldots} \\
145 & Decision Nature & \textit{I think a connection with a pet is very personal, so it evokes personal feelings\textbackslash\ldots} \\
147 & Interaction Attribution & \textit{That's where the ChatBot is taking me} \\
160 & Emotional Driver & \textit{The pull to feel happier is important to me} \\
178 & Thinking Style & \textit{I think I feel so strongly in the convictions of my emotions and choices} \\
184 & Self-Diagnosed Focus & \textit{It's because the issues predominantly arise from internal changes. The external \textbackslash\ldots} \\
220 & Emotional Driver & \textit{I am experiencing a mental torment in relation to the options} \\
218 & Interaction Attribution & \textit{That chat bot has not guided the thread to this conversation} \\
219 & Interaction Attribution & \textit{the conversation was guided this way - We move from one element to the other. Th\textbackslash\ldots} \\
230 & Deliberate Prioritisation & \textit{Because other people's opinions and pressures on this subject hold no sway over \textbackslash\ldots} \\
233 & Self-Diagnosed Focus & \textit{Because I'm still working through the trauma of my childhood, it never really le\textbackslash\ldots} \\
299 & Self-Diagnosed Focus & \textit{It's the emotional part that keeps me stuck} \\
317 & Self-Diagnosed Focus & \textit{Maybe my age, personal values and life experience} \\
\bottomrule
\end{tabular*}
\end{table}

\vspace{6pt}
\noindent\textbf{Group 5:} Dominant dimension = \textit{internal}, score gap = 2, observation type = \textit{opening}. \textit{n} = 14 moments; 6 distinct taxonomy categories.

\begin{table}[!h]
\footnotesize
\centering
\begin{tabular*}{\columnwidth}{@{\extracolsep{\fill}}@{} p{0.10\columnwidth} p{0.36\columnwidth} p{0.46\columnwidth} @{}}
\toprule
\textbf{ID} & \textbf{Category} & \textbf{Interpretation (truncated)} \\
\midrule
82 & Self-Diagnosed Focus & \textit{I tend to think alot about what other people opinions are about me and how they \textbackslash\ldots} \\
105 & Content-Level Response & \textit{I think I know deep down that it's the right long term decision, but it's a gamb\textbackslash\ldots} \\
121 & Self-Diagnosed Focus & \textit{i can be quite a selfish person sometimes} \\
128 & Self-Diagnosed Focus & \textit{I feel like I have so much going on in my own head I sometimes can't take other \textbackslash\ldots} \\
179 & Self-Diagnosed Focus & \textit{I think I do focus on other people's experiences and feelings quite a lot. I pro\textbackslash\ldots} \\
183 & Deliberate Prioritisation & \textit{Because it feels like a personal decision} \\
227 & Content-Level Response & \textit{I didnt mention that its a lot harder for me to concieve because of my health co\textbackslash\ldots} \\
242 & Decision Nature & \textit{I don't know I don't think I have got past the first stage of weather I think it\textbackslash\ldots} \\
245 & Emotional Driver & \textit{I feel that I am lost and ensure what to do for the future} \\
259 & Emotional Driver & \textit{I just always try and find how my own feelings are but struggle to understand th\textbackslash\ldots} \\
260 & Thinking Style & \textit{I often like to look at all aspects and angles before making a decision, I'm not\textbackslash\ldots} \\
270 & Deliberate Prioritisation & \textit{I focused more on my feelings and goals because they felt most important at the \textbackslash\ldots} \\
286 & Decision Nature & \textit{Agree real world less explored due to financial costs than aspirational.} \\
314 & Deliberate Prioritisation & \textit{I believe that to be the best version of myself, I need to evaluate myself inter\textbackslash\ldots} \\
\bottomrule
\end{tabular*}
\end{table}
