# Supplementary material for: Why This and Not That? A Collaborative Reflection Approach for Understanding Thought Coverage in Decision Making Support Dialog
Source: arXiv:2608.17054 source file (2026-10-04)
Supplement: Supplementary file 2 [file appendix_H_examples.tex]

\section*{Appendix H: Complete Example Moments}

Four complete pause moments illustrating the three-step exchange (observation -- recognition -- interpretation -- decision). Examples were selected to represent qualitatively distinct taxonomy categories.

\paragraph{Example 1: Deliberate Prioritisation}
\begin{quote}\small
\textbf{Participant:} 70, Decision: Start a new job/position\\
\textbf{Observation:} I want to pause and share an observation. We've been working through your own past experiences, and stories or lessons from people you know, but practical constraints, other people's opinions and pres\textbackslash\{\}ldots\{\}\\
\textbf{Recognition:} Yes\\
\textbf{Interpretation:} It's because it's only the practical constraints that I can't see a clear way through. I don't mind making a fool of myself whilst I get into my stride choosing appropriate content topics and putting them into a video format that works. It's the practical constraints of doing that visibly and whether it'd create the impression I'm capable of working more than I currently am and wether it'd jeopardise my hard fought part time position.\\
\textbf{Decision chosen:} Explore your feelings, personal values, and emotions\\
\textbf{Reason:} It's the only subject we've not covered yet\\
\textbf{Agent default:} Explore your feelings, personal values, and emotions\\
\textbf{Aligned:} Yes\\
\textbf{Taxonomy category:} \textbf{Deliberate Prioritisation}\\
\end{quote}

\paragraph{Example 2: Self-Diagnosed Focus}
\begin{quote}\small
\textbf{Participant:} 64, Decision: Pursue a degree\\
\textbf{Observation:} Here is what I observed from what you shared earlier. Your reflection has focused mainly on internal aspects, such as your feelings, personal values, and emotions, while experiential aspects, such as \textbackslash\{\}ldots\{\}\\
\textbf{Recognition:} Yes\\
\textbf{Interpretation:} I think I tend to focus on the negatives, which means I initially ignore experiences of people who have successfully taken the path I aim to. I am aware of people who have pivoted their career in the same way at a similar age. I have some concerns that in my current work I will struggle to pursue a degree, and I was worried they would react negatively when I first mentioned it. I still am, but I am more concerned about staying in this role for a long time.\\
\textbf{Decision chosen:} Explore your own past experiences, and stories or lessons from people you know\\
\textbf{Reason:} I think it would benefit me to put this decision in the context of difficult decisions I've had to make in the past in order to lessen the gravity of it.\\
\textbf{Agent default:} Explore your own past experiences, and stories or lessons from people you know\\
\textbf{Aligned:} Yes\\
\textbf{Taxonomy category:} \textbf{Self-Diagnosed Focus}\\
\end{quote}

\paragraph{Example 3: Emotional Driver}
\begin{quote}\small
\textbf{Participant:} 14, Decision: Quit a job/position\\
\textbf{Observation:} Let me share what I've been noticing. Even as we explored practical constraints, other people's opinions and pressures, and real-world conditions together, your feelings, personal values, and emotions\textbackslash\{\}ldots\{\}\\
\textbf{Recognition:} Yes\\
\textbf{Interpretation:} i tend to worry a lot, about my family, especially my mum, that i can always take care of her\\
\textbf{Decision chosen:} Continue exploring your feelings, personal values, and emotions\\
\textbf{Reason:} to look at my thoughts\\
\textbf{Agent default:} Explore your own past experiences, and stories or lessons from people you know\\
\textbf{Aligned:} No\\
\textbf{Taxonomy category:} \textbf{Emotional Driver}\\
\end{quote}

\paragraph{Example 4: Pattern Disputed}
\begin{quote}\small
\textbf{Participant:} 31, Decision: Buy a home\\
\textbf{Observation:} Here is what I observed from what you shared earlier. Your reflection has lightly explored external aspects, such as practical constraints, other people's opinions and pressures, and real-world condit\textbackslash\{\}ldots\{\}\\
\textbf{Recognition:} No (alternative: I shared very surface level statement about my intent to buy a house.)\\
\textbf{Interpretation:} The recognition text seem overly verbose in relation to my reflection.\\
\textbf{Decision chosen:} Explore practical constraints, other people's opinions and pressures, and real-world conditions\\
\textbf{Reason:} There's a lot to explore in this field with logistics of buying property\\
\textbf{Agent default:} Explore your feelings, personal values, and emotions\\
\textbf{Aligned:} No\\
\textbf{Taxonomy category:} \textbf{Pattern Disputed}\\
\end{quote}
